# Supplementary material for: APT: Atomic Physical Transitions for Causal Video-Language Understanding
Source: arXiv:2606.18586 source file (2026-08-30)
Supplement: Supplementary file 1 [file 11_appendix.tex]

% ======
\newpage
\appendix
% ======

\section{Annotation Guidelines (All 14 APT Types)}
\label{app:annotation_guidelines}

For each APT type, we provide the boundary cue used by annotators.
Annotators mark the first frame where the transition is visually identifiable and the first frame where the new state is stable for three consecutive frames.
When a boundary is ambiguous, the released record includes an annotator note and is reviewed during adjudication.

\begin{table}[h]
\centering
\caption{Human annotation cues for the 14 APT types.}
\small
\begin{tabular}{@{}lp{8cm}@{}}
\toprule
\textbf{APT Type} & \textbf{Boundary cue} \\
\midrule
\texttt{contact\_init}        & Mark the first frame where two objects, or an object and a surface, visibly touch after being separated. \\
\texttt{contact\_break}       & Mark the first frame where a previously touching pair visibly separates. \\
\texttt{elastic\_rebound}     & Mark the frame where an approaching object reverses direction after impact and remains in motion. \\
\texttt{inelastic\_capture}   & Mark the transition where an impact dissipates motion and the object remains against the contacted body. \\
\texttt{free\_fall\_onset}    & Mark the first frame after support is lost and downward motion begins. \\
\texttt{projectile\_apex}     & Mark the highest visible point of an airborne trajectory before descent. \\
\texttt{landing}              & Mark first contact with a support after a fall or airborne interval. \\
\texttt{static\_breakaway}    & Mark the first frame where a previously still object begins sustained sliding. \\
\texttt{sliding\_arrest}      & Mark the first frame where a sliding object becomes stably still. \\
\texttt{surface\_transition}  & Mark the frame where an object crosses onto a new supporting surface and the support condition changes. \\
\texttt{rotation\_onset}      & Mark the first frame of sustained visible angular motion. \\
\texttt{toppling}             & Mark the frame where an object loses stability and begins falling over, not merely rocking. \\
\texttt{rotation\_arrest}     & Mark the first frame where visible rotation stops. \\
\texttt{settling}             & Mark the frame where residual wobble, bounce, or oscillation has visibly damped into stable rest. \\
\bottomrule
\end{tabular}
\end{table}

\section{Per-Type Recall on Physion++ (14-Type Portion)}
\label{app:pertype}

\begin{table}[h]
\centering
\caption{Per-type recall (\%) on the Physion++ test portion at $\pm 200$\,ms tolerance. Best zero-shot per type underlined; LoRA-v3 (specialist) and LoRA-v4 (generalist) shown for comparison. \texttt{projectile\_apex} and \texttt{inelastic\_capture} are universally 0\% under zero shot.}
\small
\resizebox{\textwidth}{!}{
\begin{tabular}{@{}l|cccc|ccc|ccc|cccc@{}}
\toprule
& \multicolumn{4}{c|}{\textbf{Contact}} & \multicolumn{3}{c|}{\textbf{Gravity}} & \multicolumn{3}{c|}{\textbf{Friction}} & \multicolumn{4}{c}{\textbf{Rotation}} \\
\textbf{Model} & \rotatebox{60}{\texttt{c\_init}} & \rotatebox{60}{\texttt{c\_break}} & \rotatebox{60}{\texttt{rebound}} & \rotatebox{60}{\texttt{capture}} & \rotatebox{60}{\texttt{ff\_onset}} & \rotatebox{60}{\texttt{apex}} & \rotatebox{60}{\texttt{landing}} & \rotatebox{60}{\texttt{breakaway}} & \rotatebox{60}{\texttt{sl\_arrest}} & \rotatebox{60}{\texttt{surf\_tr}} & \rotatebox{60}{\texttt{r\_onset}} & \rotatebox{60}{\texttt{topple}} & \rotatebox{60}{\texttt{r\_arrest}} & \rotatebox{60}{\texttt{settling}} \\
\midrule
GPT-4.1            & 32 & 28 & 20 & 0 & 6 & 0 & 22 & 8  & 14 & 1 & 9  & 11 & 7  & 4  \\
Gemini 2.5 Flash   & 30 & 26 & 18 & 0 & 4 & 0 & 20 & 6  & 12 & 1 & 8  & 9  & 6  & 3  \\
Qwen3-VL-8B        & 28 & 24 & 16 & 0 & 5 & 0 & 18 & 7  & 11 & 0 & 7  & 8  & 5  & 3  \\
InternVL3.5-2B     & 30 & 28 & 17 & 0 & 5 & 0 & 19 & 7  & 12 & 1 & 8  & 9  & 6  & 4  \\
\midrule
\texttt{APT-Tune-S}  & 75 & 70 & 60 & 25 & 35 & 18 & 55 & 40 & 50 & 30 & 38 & 45 & 36 & 28 \\
\texttt{APT-Tune-G}  & 65 & 60 & 50 & 18 & 28 & 12 & 48 & 32 & 42 & 22 & 32 & 38 & 28 & 22 \\
\bottomrule
\end{tabular}
}
\end{table}

The two universal-zero types under zero-shot (\texttt{projectile\_apex}, \texttt{inelastic\_capture}) are recovered by LoRA fine-tuning to 12 to 25\% recall, small in absolute terms but the \emph{first non-zero numbers} on these types in our setting.

\section{Training Details}
\label{app:training}

\paragraph{Data preparation.}
The APT-format SFT records are produced by
\texttt{build\_sft\_dataset.py} (specialist v3) and \texttt{build\_multiformat\_sft.py} (generalist v4).
Each APT record contains a 16-frame video reference, the prompt, and a JSON target generated from the human annotation file; MCQ and describe records contain the corresponding string target.
The chat template is uniform across formats; \texttt{format\_type} is a record-level field used by \texttt{build\_prompt()} for dispatch.

\paragraph{LoRA configuration.}
$r = 16$, $\alpha = 32$, dropout 0.0, target modules \texttt{q\_proj, k\_proj, v\_proj, o\_proj, gate\_proj, up\_proj, down\_proj}.
Vision encoder and merger are frozen.
Total trainable parameters: $\sim$11\,M.

\paragraph{Optimizer / schedule.}
AdamW, $\beta = (0.9, 0.95)$, weight decay 0.0, lr $1\!\times\!10^{-4}$, cosine schedule, 30 warm-up steps, 3 epochs over the train split.
Mixed-precision bf16, gradient checkpointing.
Single A100 (80\,GB), $\sim$22\,h end to end for v3, $\sim$30\,h for v4 (larger mix).

\paragraph{Robust JSON parser.}
At inference time, predictions sometimes truncate mid-JSON (the model emits an unterminated array because of the max-tokens limit).
We implement a tolerance-aware parser that recovers any complete leading APT records from a malformed string and discards the rest, rather than dropping the entire prediction.
This affects $<$3\% of predictions in our data but reduces variance.

\section{Evaluation Sensitivity}
\label{app:protocol}

\begin{table}[h]
\centering
\caption{Sensitivity of recall to the matching tolerance $\Delta t$ on the \aptbench{} test split. Tighter tolerance reduces recall uniformly across models; pairwise rankings are preserved.}
\small
\begin{tabular}{@{}lcccc@{}}
\toprule
\textbf{Model} & \textbf{$\Delta t = 100$\,ms} & \textbf{$\Delta t = 200$\,ms} & \textbf{$\Delta t = 300$\,ms} & \textbf{$\Delta t = 500$\,ms} \\
\midrule
Baseline 2B          & 5  & 8  & 10 & 13 \\
\texttt{APT-Tune-S}  & 38 & 46 & 50 & 53 \\
\texttt{APT-Tune-G}  & 31 & 38 & 42 & 45 \\
\bottomrule
\end{tabular}
\end{table}

\section{Audit}
\label{app:audit}

87 annotated events were independently reviewed after the main labeling pass.
Each audit item shows the source video, the labeled APT frame, the assigned type, and the involved object(s).
Coverage spans 9 of 14 APT types and both source datasets.
For each audited event, the reviewer verified that the timestamp coincides with a visually identifiable physical transition and that the label matches the definitions in Table~\ref{tab:taxonomy}.
We did not encounter a false positive in this sample; a larger double-annotation study is left to future dataset releases.

%%%%%%%%%%%%%%%%%%%%%%%%%%%%%%%%%%%%%%%%%%%%%%%%%%%%%%%%%%%%

\newpage
\section*{NeurIPS Paper Checklist}

\begin{enumerate}

\item {\bf Claims}
    \item[] Question: Do the main claims made in the abstract and introduction accurately reflect the paper's contributions and scope?
    \item[] Answer: \answerYes{}
    \item[] Justification: All claims (14-type taxonomy, $<$14\% zero-shot recall, +38\,pp APT recall / +47\,pp PhysBench / +15\,pp SSv2 MCQ) are directly supported by Section~\ref{sec:experiments}.

\item {\bf Limitations}
    \item[] Question: Does the paper discuss the limitations of the work performed by the authors?
    \item[] Answer: \answerYes{}
    \item[] Justification: Section~\ref{sec:discussion} discusses the current restriction to rigid-body and force-mediated APTs, the annotation and simulation gap, and future expansion to broader physical processes.

\item {\bf Theory Assumptions and Proofs}
    \item[] Question: For each theoretical result, does the paper provide the full set of assumptions and a complete (and correct) proof?
    \item[] Answer: \answerNA{}
    \item[] Justification: This is an empirical benchmark + method paper. The APT definition is a formalization, not a theorem.

\item {\bf Experimental Result Reproducibility}
    \item[] Question: Does the paper fully disclose all the information needed to reproduce the main experimental results?
    \item[] Answer: \answerYes{}
    \item[] Justification: Section~\ref{sec:eval_protocol} specifies the zero-shot protocol; Section~\ref{sec:method} and Appendix~\ref{app:training} specify the LoRA recipe; data sources and splits are fully enumerated.

\item {\bf Open access to data and code}
    \item[] Question: Does the paper provide open access to the data and code?
    \item[] Answer: \answerYes{}
    \item[] Justification: We release the merged \aptbench{} human annotation file, annotation guidelines, the multi-format SFT mix, the LoRA training script, and the evaluation script.

\item {\bf Experimental Setting/Details}
    \item[] Question: Does the paper specify all the training and test details?
    \item[] Answer: \answerYes{}
    \item[] Justification: Frame counts, prompts, matching tolerance, LoRA hyperparameters, and SFT data-mix sizes are specified in Sections~\ref{sec:eval_protocol}, \ref{sec:method}, and Appendix~\ref{app:training}.

\item {\bf Experiment Statistical Significance}
    \item[] Question: Does the paper report error bars suitably and correctly defined?
    \item[] Answer: \answerYes{}
    \item[] Justification: Pairwise comparisons between baseline and fine-tuned models pass paired bootstrap tests at $p < 0.001$ ($n = 1{,}000$ resamples).

\item {\bf Experiments Compute Resources}
    \item[] Question: Does the paper provide sufficient information on compute resources?
    \item[] Answer: \answerYes{}
    \item[] Justification: Each LoRA run fits on a single A100 in $\leq$30\,h. Zero-shot evaluation of all open-source VLMs takes $\sim$2 GPU-days total. API model usage is reported per-call.

\item {\bf Code Of Ethics}
    \item[] Question: Does the research conform with the NeurIPS Code of Ethics?
    \item[] Answer: \answerYes{}
    \item[] Justification: All source data is publicly released by the original authors (CLEVRER, Physion++, SSv2, PhysBench, VideoPhy2). No personal data is collected.

\item {\bf Broader Impacts}
    \item[] Question: Does the paper discuss broader impacts?
    \item[] Answer: \answerYes{}
    \item[] Justification: \aptbench{} is a diagnostic + training-target benchmark for physics understanding in VLMs, with downstream relevance to robotics, scientific video analysis, and physics-aware video generation. No direct negative societal impacts identified.

\item {\bf Safeguards}
    \item[] Question: Does the paper describe safeguards for responsible release?
    \item[] Answer: \answerNA{}
    \item[] Justification: \aptbench{} evaluates physics transition detection and poses no meaningful misuse risk.

\item {\bf Licenses for existing assets}
    \item[] Question: Are existing assets properly credited with licenses mentioned?
    \item[] Answer: \answerYes{}
    \item[] Justification: CLEVRER, Physion++, SSv2, PhysBench, VideoPhy2, Qwen3-VL, and InternVL3.5 are cited; all are released under permissive research licenses.

\item {\bf New Assets}
    \item[] Question: Are new assets well documented?
    \item[] Answer: \answerYes{}
    \item[] Justification: Dataset documentation, annotation guidelines, audit description, and recipe scripts are provided in supplementary material.

\item {\bf Crowdsourcing and Research with Human Subjects}
    \item[] Question: Does the paper include full instructions given to participants?
    \item[] Answer: \answerYes{}
    \item[] Justification: Appendix~\ref{app:annotation_guidelines} gives the APT labeling instructions and boundary cues. Annotators label public simulation videos only; no personal or behavioral data about annotators is collected.

\item {\bf Institutional Review Board (IRB) Approvals}
    \item[] Question: Does the paper describe potential risks to study participants?
    \item[] Answer: \answerNA{}
    \item[] Justification: The human work is video annotation of public non-human simulation clips, with no intervention and no collection of personal data.

\end{enumerate}
